# Supplementary material for: Topo4D: Topology-Preserving Gaussian Splatting for High-Fidelity 4D Head Capture
Source: arXiv:2406.00440 source file (2024-07-15)
Supplement: Supplementary file 1 [file method_to_supp.tex]

\input{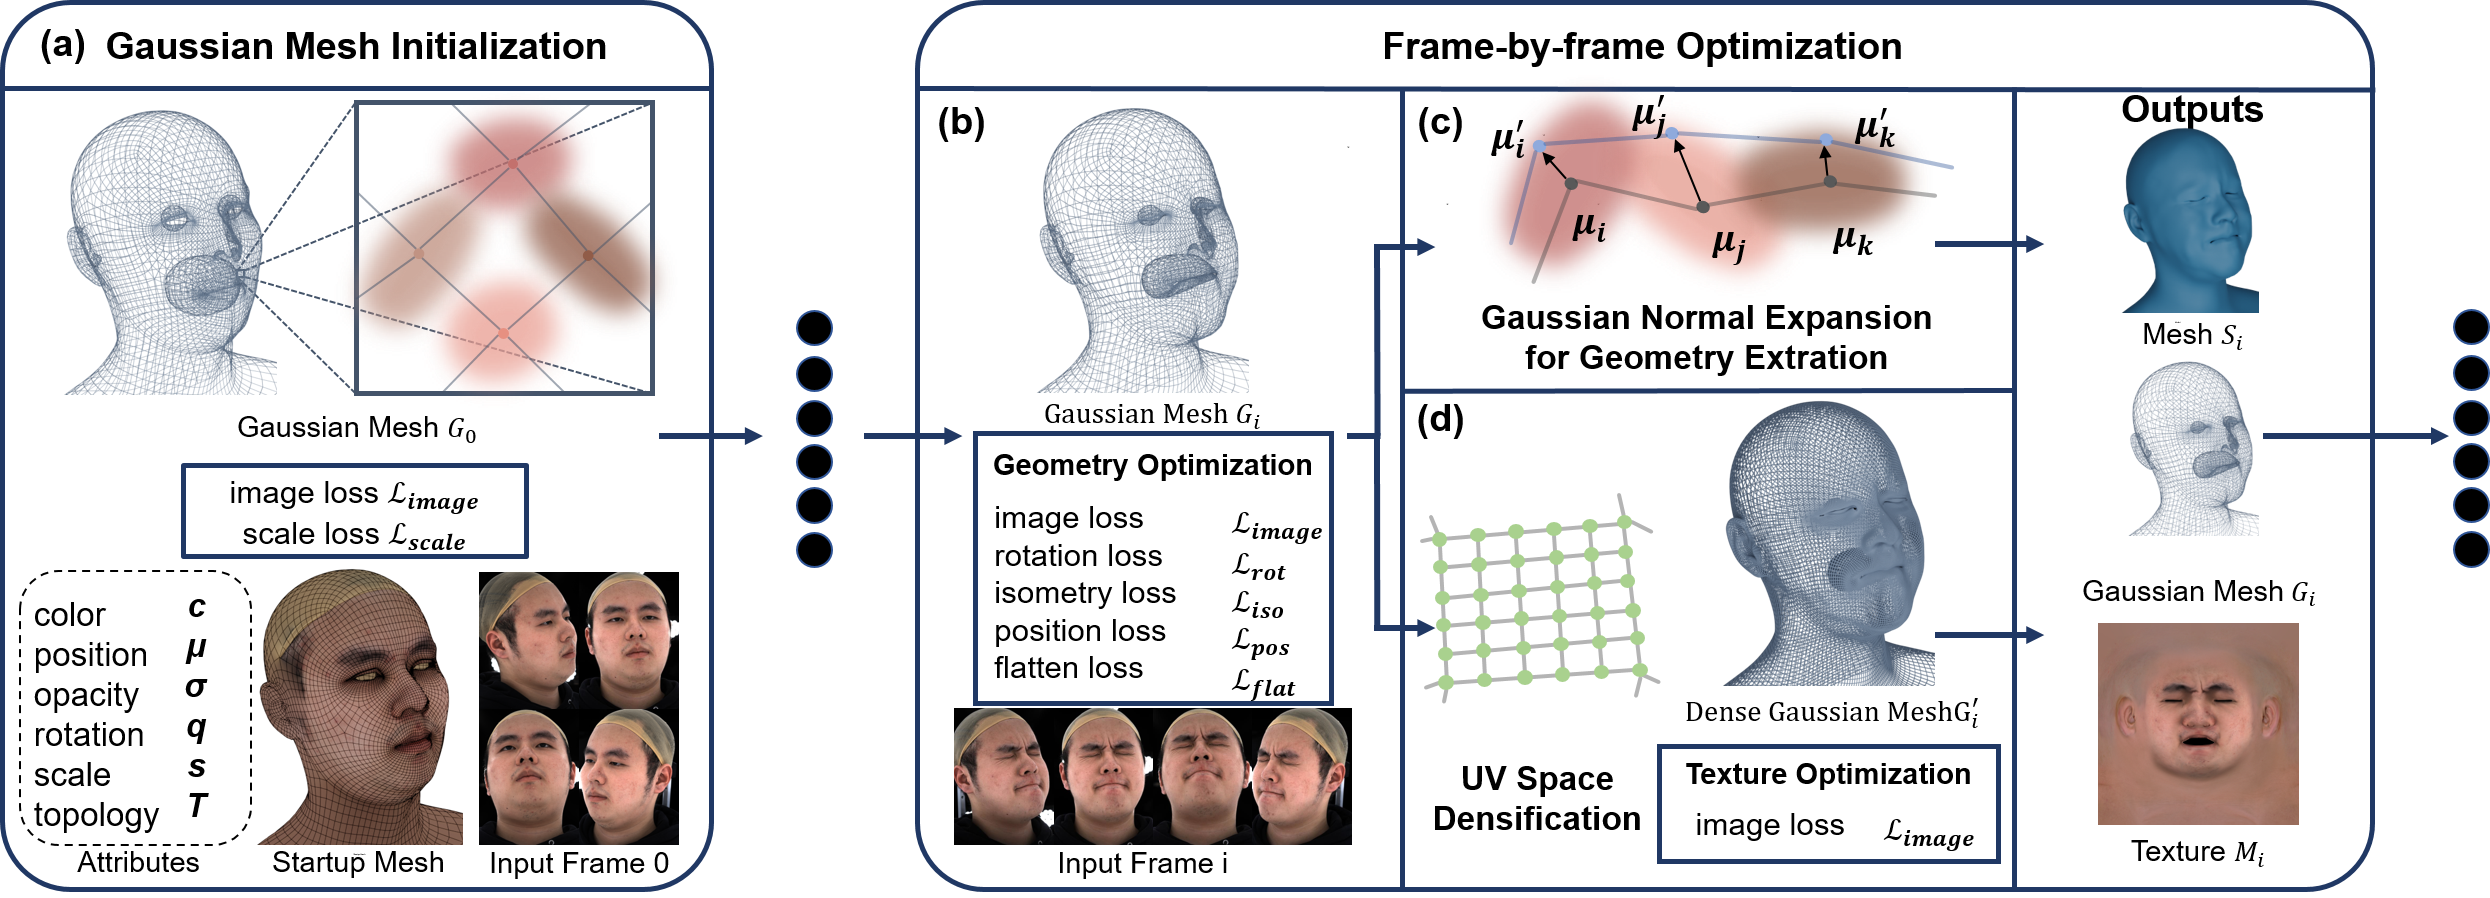}

\section{Methods}
% \indent{\it Overview.} 
Our method aims to achieve temporal stable facial mesh reconstruction and texture recovery from calibrated multi-view videos. Specifically, given sets of multi-view image sequences $\{ \mathbf{I}^j_i \in \mathbb{R}^{h \times w \times 3} | 1 \leq i \leq F\}_{j=1}^K$ in the resolution of $h \times w$, encompassing $F$ frames captured from $K$ different viewpoints, all with known camera calibrations, our method can extract head meshes 
$\{\mathbf{S}_i:=(V^i, T)|V^i\in\mathbb{R}^{n_v\times3} \}_{i=1}^F$ in the pre-defined fixed topology $T$ together with 8K texture maps $\{\mathbf{M}_i\in\mathbb{R}^{8196\times8196\times3} \}_{i=1}^F$, where $n_v$ represents the number of vertices.

To begin with, we give a brief review of 3D Gaussian Splatting~\cite{3DGS}~(Sec.~\ref{sec:Preliminary}). As illustrated in Figure~\ref{fig:dense_pic}, our method first builds a \textit{Gaussian Mesh} by initializing a topology-integrated gaussian set based on the facial priors in the first frame~(Sec.~\ref{sec:Gaussian Mesh}). Then, for each subsequent frame, we alternatively perform geometry optimization and texture optimization, to learn dynamic high-fidelity geometries and textures~(Sec.~\ref{sec:GTO}).
% by regularizing vertex motion through topology and physics-aware loss items and learn dense texture colors by UV space Gaussian densification 
Finally, we introduce how to extract geometries from \textit{Gaussian Mesh} and recover ultra high-resolution texture maps~(Sec.~\ref{sec:GTE}).
% Overview：我们的方法基于4DGS优化，输入是一组多视角视频及其相机参数，同时还有通过MVS+Registration方法生成的第一帧人脸几何和贴图。我们用第一帧的贴图和几何初始化高斯点集来构建Gaussian Mesh，为后续的优化过程提供了充分的拓扑、形状和颜色先验。通过物理和拓扑约束，我们优化并跟踪每个高斯点在每一帧的三维位置，从而提取出动态几何。在每一帧我们进行几何和纹理的交替优化，通过UV空间顶点稠密化，我们可以学习精确的顶点颜色并生成原生8K纹理。接下来我们首先介绍GS的前置知识，再给出第一帧初始化并优化Gaussian Mesh的方法。之后我们将详细介绍后续每一帧对几何和纹理的交替优化方法。
\subsection{Preliminary}
\label{sec:Preliminary}
3D Gaussian Splatting (3DGS)~\cite{3DGS} is proposed as a competitive solution for photo-realistic rendering. 
Different from other implicit methods, 3DGS explicitly maintains a set of Gaussian distributions to model a scene. 
% By virtue of the explicit intrinsics of Gaussians and the absence of dense MLP execution when sampling from scene representation, 3DGS can render scenes effciently while maintaining high fidelity. 
In 3DGS, each ellipsoidal Gaussian features a learnable color compone{nt $c$} and an opacity component $\bm{\sigma}$, and is described by a covariance matrix $\Sigma$ and its mean position {$\bm{\mu}$}:
\begin{equation}
G(\bm{x})=e^{-\frac{1}{2} (\bm{x})^T\Sigma ^{-1}(\bm{x})},
\end{equation} 
% TIn order to ensure positive definiteness of the covariance matrix to guarantee its 
% To ensure positive definiteness during the optimization process, 
where $\Sigma$ is further decomposed into rotation matrix $R$, parameterized with a quaternion $\bm{q}$, and scaling matrix $S$ :
\begin{equation}
\Sigma=RSS^TR^T.
\end{equation} 
% where $R$ is parameterized with a quaternion $q$ for the sake of optimization convenience. 

% During rendering, all 3D Gaussians are projected to 2D image plane~\cite{zwicker2001ewa}:
% \begin{equation}
% \Sigma^\prime=JW\Sigma W^TJ^T,
% \end{equation}
% where $W$ represents the viewing transformation matrix and $J$ denotes the Jacobian of the affine approximation of the projective transformation. 
In rendering, the color $\bm{C}$ of a pixel is acquired by sampling and blending all Gaussians that overlap the pixel 
in depth order: 
\begin{equation}
\bm{C}=\sum_{i=1}\bm{c}_i\alpha_i\prod_{j=1}^{i-1}(1-\alpha_i),
\end{equation} 
where the blending weight $\alpha_i$
is given by evaluating a 2D Gaussian with its covariance multiplied by its opacity.

However, 3DGS is designed for realistic rendering instead of 3D reconstruction. 
Gaussians lack inherent topological relationships, thus unconstrained optimization of their attributes may only yield irregular geometry. As a result, directly extracting topologically sound meshes becomes unfeasible.
% There is no topological relationship between Gaussians, and unconstrained optimization of their attributes can only produce meaningless geometry, making it impossible to directly extract topologically good meshes.
% Preliminary：GS能从带有位姿的多视角图进行快速高分辨率渲染，通过在第一帧优化高斯的属性，并在后续帧约束这些属性，可以通过多视角图像的变化驱动这些高斯点；{Gaussian Splatting的符号、表示、投影、渲染方程；}
% GS的优势
% GS通过分布在空间中的Gaussian混合颜色实现渲染，然而高斯点之间没有拓扑关系，不加约束地优化三维坐标会导致没有意义的几何形状，无法直接提取拓扑好的mesh和texture；

\subsection{Gaussian Mesh for Topology Integrated Gaussians Initialization}
\label{sec:Gaussian Mesh}
% Our goal is to directly extract geometry with consistent topology from Gaussians and its main challenge is the absence of topological constrains in the gradient descent optimization process. Our insight is that Gaussians can render images that reflect the head shape while maintaining topological relationships, so that we can drive Gaussians with topology by multi-view videos. We achieve this by propose \textit{Gaussian Mesh}, novelly integrating topological priors to the initialization and subsequent frame by frame optimization process of vanilla Gaussians. 

Extracting topologically consistent meshes from Gaussians is challenging due to the lack of geometric constraints during optimization.
To this end, we propose \textbf{Gaussian Mesh}, which uniquely incorporates the topological prior into vanilla Gaussian and will not affect its high-fidelity rendering quality.
% To build a Gaussian Mesh consist of two steps: \textbf{Facial Shape Binding} and \textbf{Facial Color Occupying}.
We define 4D Gaussian Meshes as $G_i=\{G_{i,j}\}_{j=1}^{n_v}$ for the $i$-th frame, where $G_{i, j}$ covers some learnable parameters, \ie, $\{\bm{\mu}_{i, j} \in \mathbb{R}^{3}, \bm{q}_{i, j} \in \mathbb{R}^{4}, \bm{s}_{i, j} \in \mathbb{R}^{3}, \bm{c}_{i, j} \in \mathbb{R}^{3}, \bm{\sigma}_{i, j} \in \mathbb{R}\}$ for the position, rotation, scaling, color, and opacity separately of the $j$-th vertice in pre-defined topology $T$.
% \todo{Sup. Mat. Attribute table}

% We first bind Gaussians to the underlying head surface. 
Different from 3DGS using SFM-generated messy sparse points for initialization, to directly obtain pre-defined topological information, we first initialize Gaussian Mesh with head mesh and texture of the first frame, which is acquired by automatic MVS and ICP algorithms. Specifically, we set the mean positions $\bm{\mu}_0$ of Gaussians to the corresponding 3D coordinates of vertices in topological order. Furthermore, 
to better align Gaussians with the surface, we initialize the orientation $\bm{q}_0$ of each Gaussian with the normal direction of vertices. 
It is worth noting that recent GaussianAvatar~\cite{GaussianAvatar} also rigs Gaussians to face model, but it is fundamentally different from our method. GaussianAvatar amis at driving Gaussians with parametric models for photo-realistic rendering, where meshes are pre-defined instead of learned.
In contrast, our goal is to extract high-quality topologic meshes and textures from multi-view videos. 
Moreover, the methods of blinding Gaussians with meshes in ours and GaussianAvatar are different. 
% meshes are vertices one by one while maintaining topological relationships, rather than attaching unstructured Gaussians to mesh surface.

% At the same time, in order to avoid color blending between multiple Gaussians as much as possible, and to form a one-to-one correspondence between the facial region and the Gaussians, we initialize the scales $s$ as half of the minimum distance between each vertex and its one-ring neighbors ($ORN$), and set opacity $\sigma$ to 1. All in all, the proposed Gaussian Mesh is composed of a set of constrained optimized Gaussians as shown in Tab. \ref{tbl:attributes}.
% Topology Integrated Gaussians initialization：与普通的3DGS使用SFM产生的稀疏点云初始化高斯点集不同，我们首先用传统MVS+Fitting的方式重建出第一帧的mesh和texture作为拓扑和颜色先验，再将Gaussian分布绑定到第一帧的人脸网格。由于希望能够从高斯点的位置直接提取出几何，我们创建与网格顶点数目相同的高斯点，将高斯的mean position按照拓扑顺序设置为网格顶点坐标；同时为了尽可能避免多个高斯间的颜色混合，使面部区域与高斯点集尽可能构成一一对应，我们将scale初始化为每个顶点与其one-ring neighbour距离的最小值，并设置每个高斯的opacity为1；

After initializing the shape-related attributes ($\bm{\mu}_0$ and $\mathbf{q}_0$) of Gaussians, we then optimize their rendering-related attributes ($\bm{s}_0$, $\bm{c}_0$ and $\bm{\sigma}_0$).
% through \textbf{Facial Color Occupying}.
% \todo{}Notably, GaussianAvatar~\cite{GaussianAvatar} also utilizes face priors by rigging Gaussians to explicit head mesh, and drive it by FLAME\cite{FLAME} parameters. However \cite{GaussianAvatar} rigs multiple Gaussians to mesh faces while we bind a single Gaussian to each vertex and build a a one-to-one mapping between Gaussians and vertices according to the topology. 
% \indent{\it Facial Color Occupying.}The logic behind facial color occupying is to make each Gaussian represent a small region of the face independently, so that the movement of the face in the videos can reflect the movement of the corresponding Gaussians. To achieve this, 
Concretely, we initialize the scales $\bm{s}_0$ as half of the minimum distance between each Gaussian and its one-ring neighbors~(ORN) and set opacity $\bm{\sigma}_0$ to 1, to avoid color blending between multiple Gaussians. To faithfully represent the color, we also initialize the color $\bm{c}_0$ of each Gaussian by sampling the corresponding pixel on the texture map according to the UV coordinate.
% Since the texture map provides the ground-truth color of the head, we set each Gaussian's color by sampling from the texture map according to the UV coordinate of each vertex. 
Finally, to learn more details in dense parts, \eg, eyes and mouth, we optimize Gaussian's rotation $\bm{q}'_0$ and scale $\bm{s}'_0$ between the first frames $\mathbf{I}_0$ and rendered images $\mathbf{I}'_0$ with the same loss function as 3DGS:
\begin{equation}
    \label{loss:image}
    \mathcal{L}_{image} = (1-\lambda ) \mathcal{L}_{1}(\mathbf{I}_0,\mathbf{I}'_0) + \lambda\mathcal{L}_{D-SSIM}(\mathbf{I}_0,\mathbf{I}'_0),
\end{equation} 
where $\lambda$ is set to 0.2. Only $\mathbf{\mu}_0$, $\mathbf{c}_0$, and $\mathbf{\sigma}_0$ are learnable during this process.

However, Gaussian is like an ellipsoid with volume, therefore a certain gap exists between the center of Gaussian and the true surface. 
% does not represent the true position of the surface it renders. 
To fill this gap, the thickness of the Gaussian in the normal direction should be as small as possible.
% If we want to extract geometry from Gaussians, we need to hypothesize that the Gaussians are like flat ellipses and aligned with the underlying head surface closely. 
Therefore, we propose a scale loss to limit the thickness of the Gaussians and penalize Gaussians with a scale exceeding $\lambda_{init}$ times than the initial value $\bm{s}_0$:
\begin{equation}
    \mathcal{L}_{scale} = \sum_{i\in G}(\Vert \bm{s}'_0 \Vert_{-\infty} + max(0, \bm{s}'_0 -\lambda_{init} \bm{s}_0)).
\end{equation} 
% where Gaussian with scale exceeding 1.5 times the initial value $\bm{s}_0$ will be penalized.

Overall, the final loss to initialize Gaussian Mesh can be formulated as:
\begin{equation}
    \mathcal{L}_{init} = \mathcal{L}_{image} + \lambda_{scale} \mathcal{L}_{scale}.
\end{equation}
% 初始帧优化目标：由于已知第一帧的可靠几何和颜色先验，因此我们在第一帧只优化高斯的scale、rotation。初始帧优化阶段使用和3DGS相同的image损失（L1loss + ssim）:{公式和说明}
%scale损失：{公式和说明}
%接下来我们具体介绍后续帧的几何优化。

\subsection{Alternative Geometry and Texture Optimization}
\label{sec:GTO}
After initializing Gaussian Mesh $G_0$, we propose an \textbf{Alternative Geometry and Texture Optimization method} to acquire Gaussian Mesh $G_i$ at frame $i$ from $G_{i-1}$.
Specifically, we optimize geometry by driving Gaussians under the regularization of topology and physics. Additionally, dense texture can be learned based on the current geometry.

\subsubsection{Geometry Optimization.}\label{sec:geo opt} 
Naively optimizing Gaussian Mesh will cause topological confusion. To maintain the topology relationships within Gaussians and regular mesh arrangement, we extend 3DGS by introducing physical and topological priors to the optimization objectives.

Specifically, we propose physical loss item $\mathcal{L}_{phy}$ that constrain local rigidity and topological loss $\mathcal{L}_{topo}$ that improve the mesh quality.

Overall, the loss items for geometry optimization is constructed by three parts: \begin{equation}
    \mathcal{L}_{geo} = \mathcal{L}_{image} + \mathcal{L}_{phy} + \mathcal{L}_{topo},
\end{equation} where the image loss is illustrated as Eq. \ref{loss:image}.
%通过在第一帧用可靠先验初始化高斯的rgb/position，同时设置opacity为1，可以使得每个3D高斯表示人脸相应位置的物理成分；通过在后续帧限制高斯scale，同时放开rotation和position、可以建模人脸相应物理成分的运动。
% 值得注意的是，相同的面部区域会随着表情的不同产生不同的阴影颜色，因此我们放开rgb的学习，有助于建模由于人脸动态运动导致的阴影和褶皱。第一帧的面部颜色先验无法给予这部分信息，但是对识别人脸几何十分重要。

\indent{a) Physical Prior Loss.} The correspondence between Gaussians and facial regions achieved by color similarity is weak. For example, for regions such as forehead and cheek, where the color is similar and the geometry is relatively flat, a Gaussian can freely represent similar physical areas, leading to incorrect tracking relationships. This means that in addition to indirectly optimizing Gaussian positions through differentiable rendering, physical priors are needed to regularize the motion of Gaussians directly. Following the practice of \cite{DynamicGaussian} but with some modifications, we regularize short-term rotation
similarity and long-term local isometry between Gaussians. 
%We refer readers to \cite{DynamicGaussian} for more details about the original design of these loss terms.

% 只通过冻结高斯的部分属性来实现高斯和人脸对应位置的绑定是不可靠的，例如对于额头、脸颊等区域，颜色相同且几何较为平整，一个高斯可以自由地表征相似的物理区域，导致错误的跟踪关系。
The physical loss between Gaussians should under the priors of topology for we don't want a Gaussian to affect all nearby Gaussians blindly, e.g. a Gaussian on the upper lip and a Gaussian on the lower lip but closest to it. Therefore, unlike \cite{DynamicGaussian}, we only impose such loss between one-ring neighbours:
% \begin{equation}
%     \mathcal{L}_{rigid}(i, j)=w_{i, j}\Vert(\mu_{j,t-1}-\mu_{i,t-1})-R_{i,t-1}R_{i,t}^{-1}(\mu_{j,t}-\mu_{i,t})\Vert_2
% \end{equation}
% \begin{equation}
%     \mathcal{L}_{rigid}=\frac{1}{2n_e} \sum_{i\in G}\sum_{j\in ORN_i} \mathcal{L}_{rigid}(i,j)
% \end{equation}, where $n_e$ is the number of edges and $ORN_i$ means the one-ring neighbours of $G_i$. The loss weighing factor takes into account the edge length of the Gaussian Mesh at the first frame:\begin{equation}
%     w_{i, j}=exp(-\lambda_w\Vert\mu_{j, 0}-\mu_{i,0}\Vert_2^2).
% \end{equation}

% % 刚体距离损失：{公式和说明}
% We also regularize Gaussian's rotation in a similar manner:
\begin{equation}
     \mathcal{L}_{rot}=\frac{1}{2n_e} \sum_{i\in G}\sum_{j\in ORN_i} w_{i,j}\Vert\bm{\hat q}_{j, t}\bm{\hat q}_{j, t-1}^{-1}-\bm{\hat q}_{i, t}\bm{\hat q}_{i, t-1}^{-1}\Vert_2,
\end{equation} where $\bm{\hat q}$ is the normalized quaternion, $n_e$ is the number of edges, and $ORN_i$ means the one-ring neighbours of $G_i$. The loss weighing factor takes into account the edge length of the Gaussian Mesh at the first frame:\begin{equation}
    w_{i, j}=exp(-\lambda_w\Vert\bm{\mu}_{j, 0}-\bm{\mu}_{i,0}\Vert_2^2).
\end{equation}

% 刚体旋转损失：{公式和说明}
In addition to the rotation similarity calculated between adjacent frames, we find that long-term physical loss is important for maintaining long-term presentation consistency:\begin{equation}
    \mathcal{L}_{iso}=\frac{1}{2n_e} \sum_{i\in G}\sum_{j\in ORN_i} w_{i,j}|\Vert\bm{\mu}_{j,0}-\bm{\mu}_{i,0}\Vert_2-\Vert\bm{\mu}_{j,t}-\bm{\mu}_{i,t}\Vert_2|.
\end{equation}

Finally, our physical loss items can be defined as:\begin{equation}
    \mathcal{L}_{phy} = \lambda_{rot}\mathcal{L}_{rot} + \lambda_{iso}\mathcal{L}_{iso}.
\end{equation}

% 刚体长距离损失：{公式和说明}
\indent{b) Topology Prior Loss.} By means of the physical constraints mentioned above, our method is able to achieve long-term tracking of the corresponding face regions. But if vertices are strictly constrained by physical constraints, it can lead to bad wiring and unsmooth surfaces. Therefore, we introduce topological priors to regularize vertex motion. Specifically, we consider both the distance constraint between each vertex and its one-ring neighbours, as well as the angle constraint between each face and its adjacent faces.

% 尽管通过上述的物理约束，已经可以实现高斯对人脸相应区域的长距离跟踪。但如果完全严格地让顶点遵从物理约束，会导致个别表情出现顶点的聚集现象。虽然符合物理实际，但是不利于生成良好的网格。{举例说明}。因此顶点的优化还需要考虑拓扑先验。

% Firstly, we constrain each edge to keep a similar proportion among all connected edges of each vertex:\begin{equation}
% \begin{split}
%     \mathcal{L}_{norm} = \frac{1}{2n_e}\sum_{i\in G}\sum_{j\in ORN_i}|\frac{\Vert\mu_{i,t}-\mu_{j,t}\Vert_2}{\sum_{k\in ORN_i}\Vert\mu_{i,t}-\mu_{k,t}\Vert_2}\\
% -\frac{\Vert\mu_{i,0}-\mu_{j,0}\Vert_2}{\sum_{k\in ORN_i}\Vert\mu_{i,0}-\mu_{k,0}\Vert_2}|.
% \end{split}
% \end{equation}

% %，我们通过初始帧网格中每个顶点的边长等比例来体现这种先验约束。
% % 边长比例损失：{公式和说明}
% We find that the above constraints alone cannot guarantee a smooth mesh. We further apply mesh flattening loss\cite{SoftRas} to the geometry to improve mesh quality:\begin{equation}
%     \mathcal{L}_{flat} = \sum_{\theta_i \in e_i}(cos\theta_i+1)^2,
% \end{equation} where $\theta_i$ is the angle between the faces that have the common edge $e_i$. This loss term effectively prevents self-intersection and make the mesh smooth enough.

To prevent the vertices from moving freely, we calculate L2 loss between the position of each vertex and the average position of its neighbours:\begin{equation}
    \mathcal{L}_{pos}=\frac{1}{n_v}\sum_{i\in G}(\bm{\mu}_i-\frac{ {\textstyle \sum_{j\in ORN_i}\bm{\mu}_j} }{|ORN_i|} )^2
\end{equation}

We further apply mesh flattening loss to encourage the angle between adjacent faces to remain constant with the first frame during the optimization process:\begin{equation}
    \mathcal{L}_{flat} = \sum_{\theta_i \in e_i}(1-cos(\theta_{i,t}-\theta_{i,0})),
\end{equation} where $\theta_{i,t}$ is the angle between the faces that have the common edge $e_i$ at frame t. This loss term effectively prevents self-intersection and make the mesh smooth enough.

Overall,  our topological prior loss consists of two parts:\begin{equation}
    \mathcal{L}_{topo} = \lambda_{pos}\mathcal{L}_{pos} + \lambda_{flat}\mathcal{L}_{flat}.
\end{equation}

% \indent{c) Optimizing Strategy.} By freezing the scale in subsequent frames while releasing rotation and position, the motion of the corresponding physical components of the face can be modeled. It is worth noting that the same facial region will present different color when doing different expressions, e.g. ambient occlusion around wrinkles. By allowing Gaussian's color change, we can to some extent model shadows caused by self occlusion, which is crucial for recognizing facial geometry. We optimize color and freeze other attributes only in the last 100 iterations of each frame.
%我们发现仅仅通过上述约束并不能保证可以从高斯集合提取平滑的网格，我们进一步对几何施加网格平滑损失来提高网格质量。
% 平滑损失：{公式和说明}
% 综上所述：topo loss = edge_norm loss + flat loss

\subsubsection{Texture Optimization}\label{sec:tex opt} After geometry optimization, we have obtained the geometry of each frame, and also the color of each Gaussian that can represent the head coarsely. Compared to representing geometry, representing pore-level details and generating 8K texture map requires more Gaussians learning on 4K images. 3DGS adopts an adaptive densification and pruning process, allowing the density of Gaussians to adaptively change with the complexity of the underlying scene. However, due to the need to maintain topological relationships to achieve inverse texture mapping, similar densification processes cannot be used here. We thus propose a novel densification method i.e. \textbf{UV Space Densification}, which allows us to insert more Gaussians to Gaussian Mesh without destroying the topology.

\indent{a) UV Space Densification.} We build a dense Gaussian Mesh $G^{\prime}$ by inserting Gaussians to the original Gaussian Mesh $G$. It's worth noting that $G^{\prime}$ is independent with $G$ and we only optimize $G^{\prime}$ during texture optimization. Specifically, we firstly clone $G$ and only inherit their position/rgb as initialization. Then for each quadrilateral mesh grid in $G^{\prime}$, we sequentially insert totally $N \times N-4$ Gaussians ($N-2$ on each edge and $(N-2) \times (N-2)$ inside the grid). \todo{Image}The newly generated Gaussian's position, UV coordinates, and color are obtained by bilinear interpolation sampling the corresponding attributes of the four Gaussians (e.g. $G_{0, 0}^{\prime}$, $G_{0, N-1}^{\prime}$, $G_{N-1, 0}^{\prime}$ and $G_{N, N}^{\prime}$) at the grid vertices:\begin{equation}\label{eq:sampling}\begin{split}
A_{i, j} = \frac{1}{(N-1)\times (N-1)}
\begin{bmatrix}
 N-1-i & i
\end{bmatrix}\\
\begin{bmatrix}
 A_{0,0} & A_{0,N-1}\\
 A_{N-1,0} & A_{N-1,N-1}
\end{bmatrix}
\begin{bmatrix}
 N-1-j\\
 j
\end{bmatrix},
\end{split}
\end{equation} where A can be color, uv coordinates, and position. Most importantly, it is also easy to establish connection relationships between Gaussians. For example, $G_{i, j}$ is connected to $G_{i-1, j}$, $G_{i+1, j}$, $G_{i, j-1}$ and $G_{i, j+1}$. This process is actually equivalent to subdividing the grid and inserting more sampling points in UV space.

For dense Gaussian Mesh $G^{\prime}$ at frame $i$, we follow a similar pratice as we do in Sec. \ref{sec:Gaussian Mesh}. Specifically, we sampling each Gaussian's $\bm{\mu}$ by Eq. \ref{eq:sampling} and set their opacity to 1. The rotation and color are inherited from previous frame. Since we only need to learn the exact color of the UV space sampling points represented by each Gaussian, we only fix Gaussian scale to be its minimum distance with one-ring neighbours. The training objective is the same as Eq. \ref{loss:image}.

\subsection{Extracting Geometry and Texture from Gaussians}
\label{sec:GTE}
% Once alternating geometry and texture optimization is done, we can finally extract geometry from $G_i$ and extract 8K texture map from $G_i^{\prime}$.
After completing the geometry and texture optimization, we are able to extract geometry from $G_i$ and an 8K texture map from $G_i^{\prime}$.
% By extracting geometry and texture map frame by frame, our framework can generate dynamic high-fidelity head mesh together with temporal consistant ultra-high resolution texture map with pore-level details.
\subsubsection{Geometry Extraction}
The Gaussian function in 3D space corresponds to an ellipsoid. Consequently, the surface shaped by the Gaussian function differs from the geometric surface formed by the Gaussian mean position, which the Gaussian functions generally encase.
To this end, we employ a method called \textit{Gaussian Normal Expansion} to make surfaces derived from Gaussian surfaces resemble real surfaces more closely.
As illustrated in \todo{Image}, we shift each Gaussian in the direction of the vertex normal to obtain the final mesh vertices:
% Since a Gaussian is equivalent to an ellipsoid in 3D space, the surface rendered by Gaussian and the geometric surface formed by Gaussian mean positions are not the same, and the latter tends to be enveloped by the former. We perform \textit{Gaussian Normal Expansion} to make the surface extracted from Gaussians closer to the real surface. Specifically, as is shown in \todo{Image}, we offset each Gaussian along vertex normal direction to get the final mesh vertex:
\begin{equation}
        \bm{n}^{\prime} = R^{-1}\bm{n},
\end{equation} 
\begin{equation}
        \bm{\mu}^{\prime} = \bm{\mu} + \sqrt{\frac{1}{\frac{n_x^{\prime 2}}{s_x^2}+\frac{n_y^{\prime 2}}{s_y^2}+\frac{n_z^{\prime 2}}{s_z^2}} }\bm{n},
\end{equation}
where $\bm{n}$ is the corresponding vertex normal of each Gaussian.
We final compensate errors caused by Gaussian scale and obtain the topological head mesh.
% where $\bm{n}$ is the corresponding vertex normal of each Gaussian and we omit vertex numbering. Finally, we compensate for errors caused by Gaussian scale and acquire the head mesh.

\subsubsection{Texture Extraction}
% To generate 8K texture map from dense Gaussian Mesh $G^{\prime}$ is to inverse map colors according to their uv coordinates and interpolate each pixel's color. Since we also maintain the topology between Gaussians in Sec. \ref{sec:tex opt}, we can triangulate the Gaussian Mesh and then directly render the texture map using traditional rasterization based rendering. Denoting the Gaussian indices of the triangle visible in pixel $(x, y)$ by $i_{0,1,2}$, and the
% barycentrics by $w_{0,1,2}$. The pixel color at $(x, y)$ can be computed by:
To generate 8K texture maps from a dense Gaussian mesh $G^{\prime}$, we map the colors inversely based on their UV coordinates. Since our Gaussian meshes are topologized, we can triangulate them and render the texture map using traditional rasterization-based rendering. If the Gaussian indices of the visible triangles for a pixel at $(x, y)$ are denoted as $i_{0,1,2}$ and the center of mass is denoted as $w_{0,1,2}$, we can calculate the color of the pixel at $(x, y)$.
That is:
\begin{equation}
    C_{x,y}=w_0c_{i_0} + w_1c_{i_1} + (1-w_0-w_1)c_{i_2}.
\end{equation}
